# Supplementary material for: Giant Strain Tunability in Polycrystalline Ceramic Films via Helium Implantation
Source: arXiv:2409.13505 ancillary file (2025-01-23)
Supplement: Supplementary file 1 [file He_implantation_Supp.pdf]

**Supplementary material for:**

**"Giant Strain Tunability in Polycrystalline Ceramic Films via Helium Implantation"**


A. Blázquez Martínez[1,2,3], S. Glinšek[1,3], T. Granzow[1,3], J.-N. Audinot[1], P. Fertey[4], J. Kreisel[2,3], M. Guennou[2,3], and C. Toulouse[1,2,3,5a)]

[1] *Smart Materials Unit, Luxembourg Institute of Science and Technology, 41 rue du Brill, 4422 Belvaux, Luxembourg*

[2] *Department of Physics and Materials Science, University of Luxembourg, 41 rue du Brill, 4422 Belvaux, Luxembourg*

[3] *Inter-institutional Research Group Uni.lu–LIST on ferroic materials, 41 rue du Brill, 4422 Belvaux, Luxembourg*

[4] *Synchrotron SOLEIL, L'Orme des merisiers, Saint-Aubin, Gif-sur-Yvette, France*

[5] *CRISMAT Laboratory, University of Caen, CNRS UMR-6508, ENSICAEN, 6 Bd du Maréchal Juin, F-14000 Caen, France*

a) Electronic mail: constance.toulouse@cnrs.fr

## CONTENTS

I. **Bragg peaks measured on every configuration, in every implanted regions of the 4 samples.** 3

II. **Visualization of the zones from a linescan** 7

III. **Example for a fit of a diffraction pattern** 8

IV. **XRD peak widths as a function of He dose: representative examples** 9

V. **Irrelevance of a small tilt for the strain values** 12

# I. BRAGG PEAKS MEASURED ON EVERY CONFIGURATION, IN EVERY IMPLANTED REGIONS OF THE 4 SAMPLES.

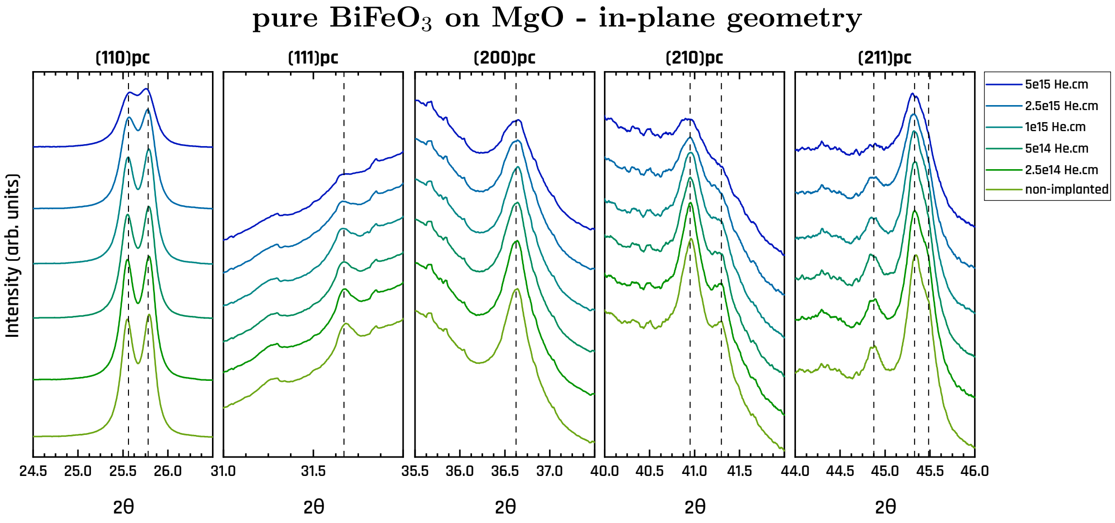


FIG. S1. Bragg Peaks measured on the pure $BiFeO_3$ film on MgO, in the in-plane configuration.

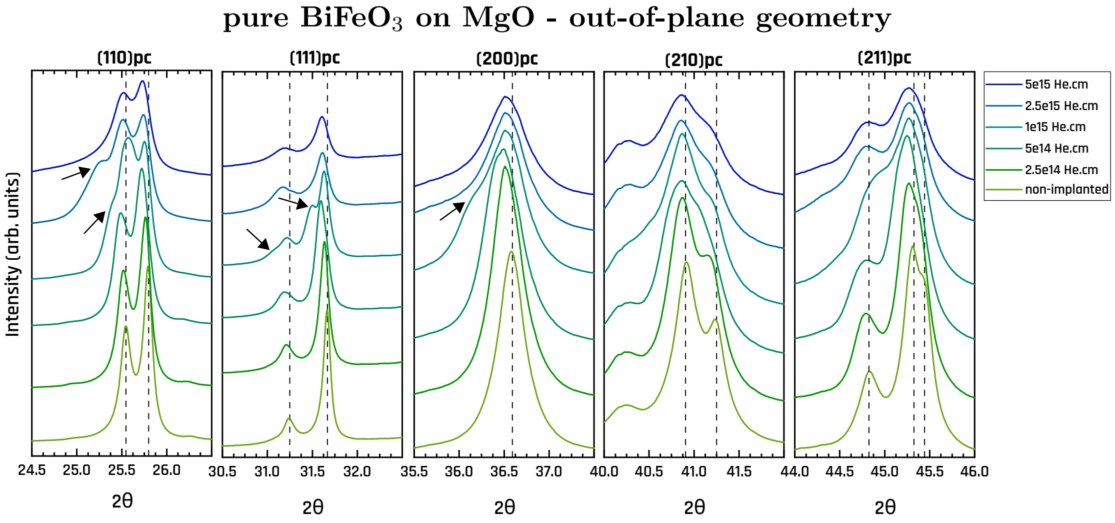


FIG. S2. Bragg Peaks measured on the pure $BiFeO_3$ film on MgO, in the out-of-plane configuration. The arrows show the appearance of the new peaks.

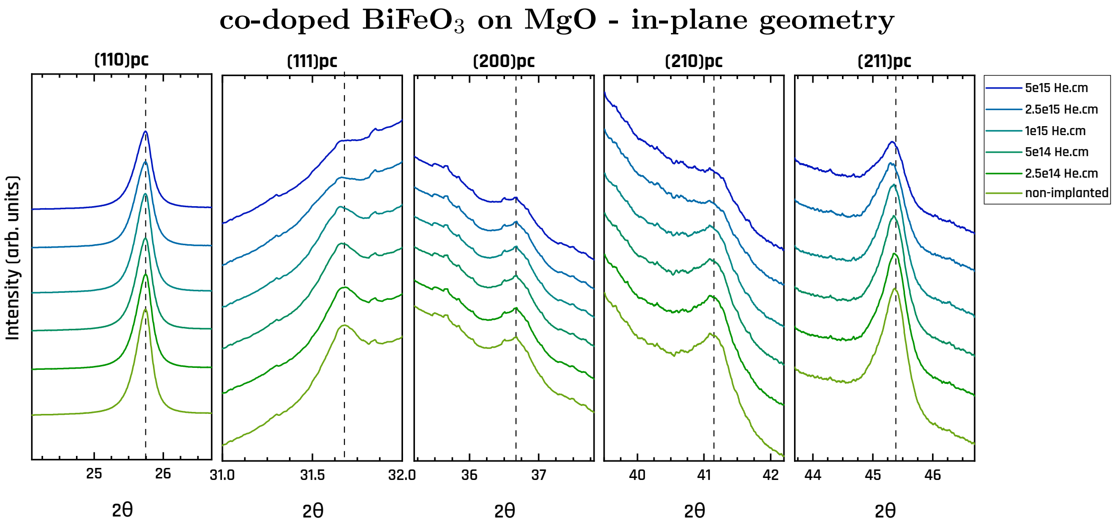


FIG. S3. Bragg Peaks measured on the co-doped $BiFeO_3$ film on MgO, in the in-plane configuration.

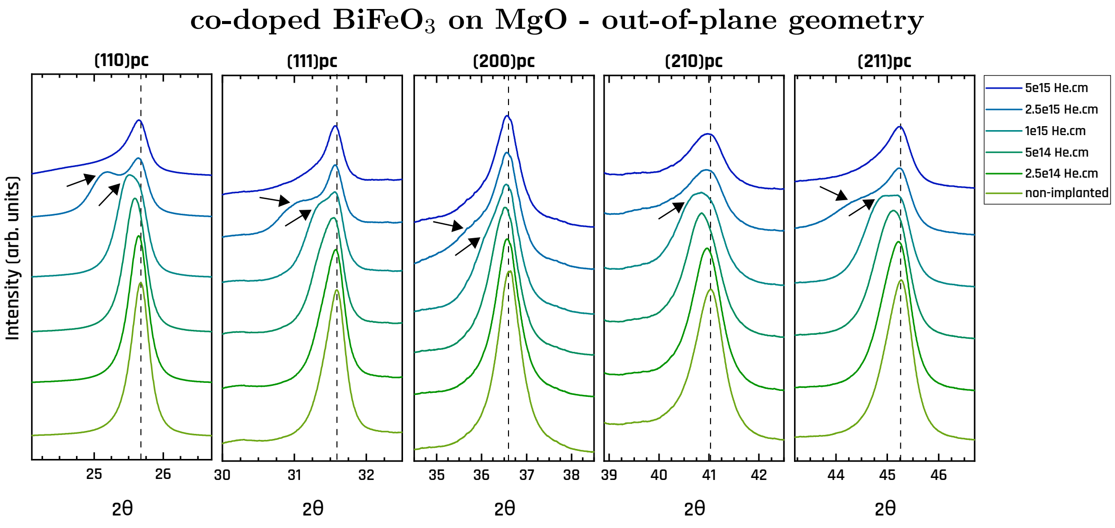


FIG. S4. Bragg Peaks measured on the co-doped $BiFeO_3$ film on MgO, in the out-of-plane configuration. The arrows show the appearance of the new peaks.

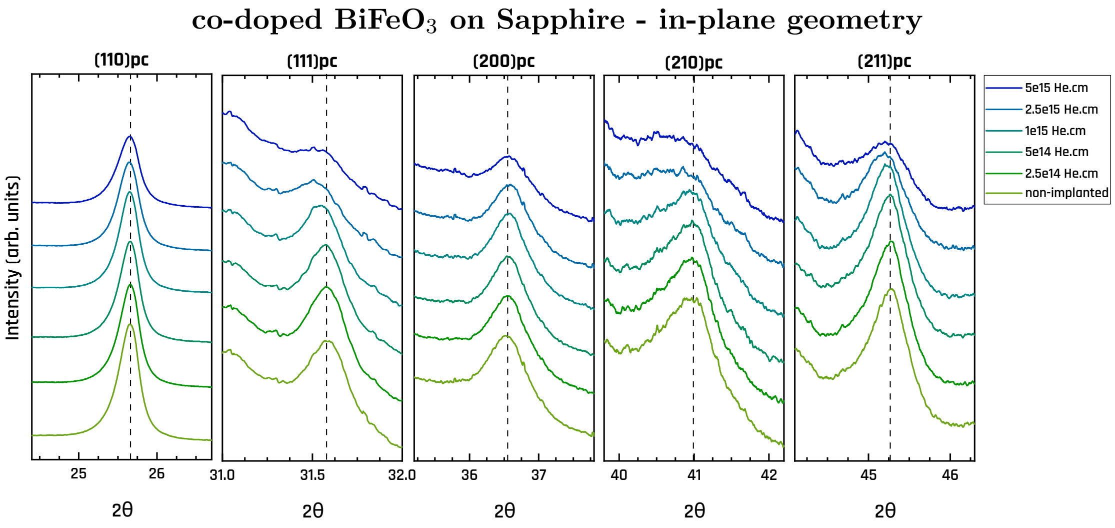


FIG. S5. Bragg Peaks measured on the co-doped $BiFeO_3$ film on Sapphire, in the in-plane configuration.

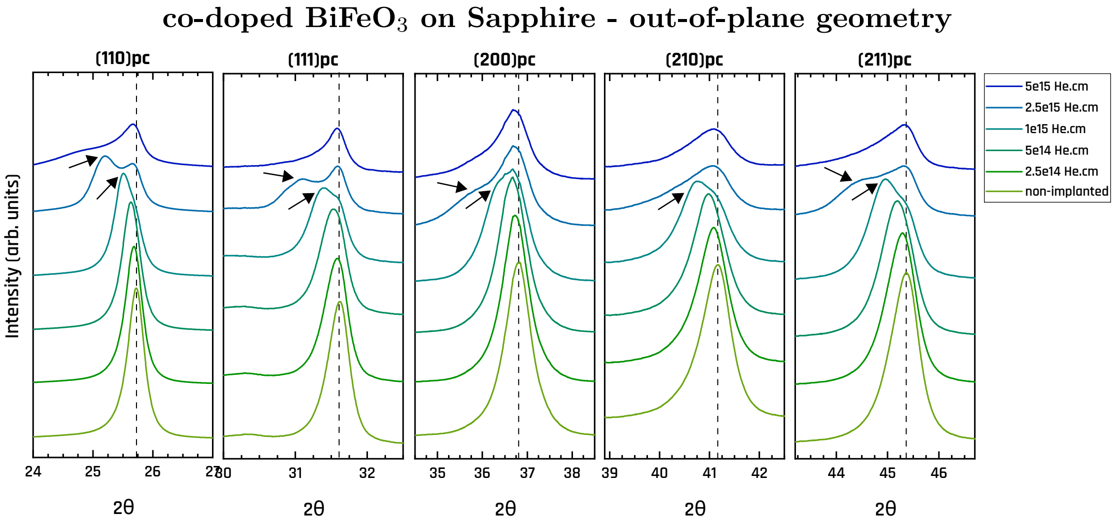


FIG. S6. Bragg Peaks measured on the co-doped $BiFeO_3$ film on Sapphire, in the out-of-plane configuration. The arrows show the appearance of the new peaks.

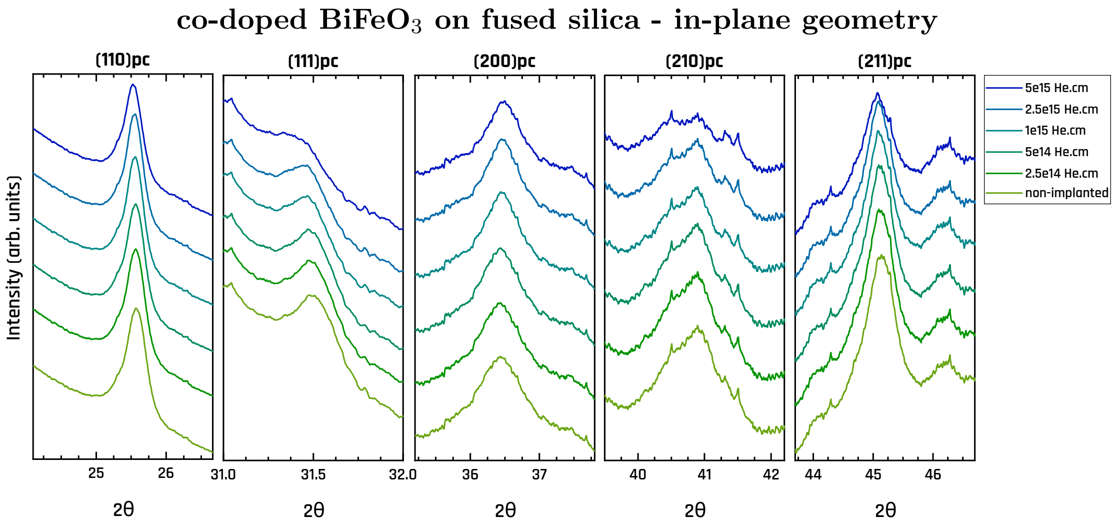


FIG. S7. Bragg Peaks measured on the co-doped $BiFeO_3$ film on fused silica, in the in-plane configuration.

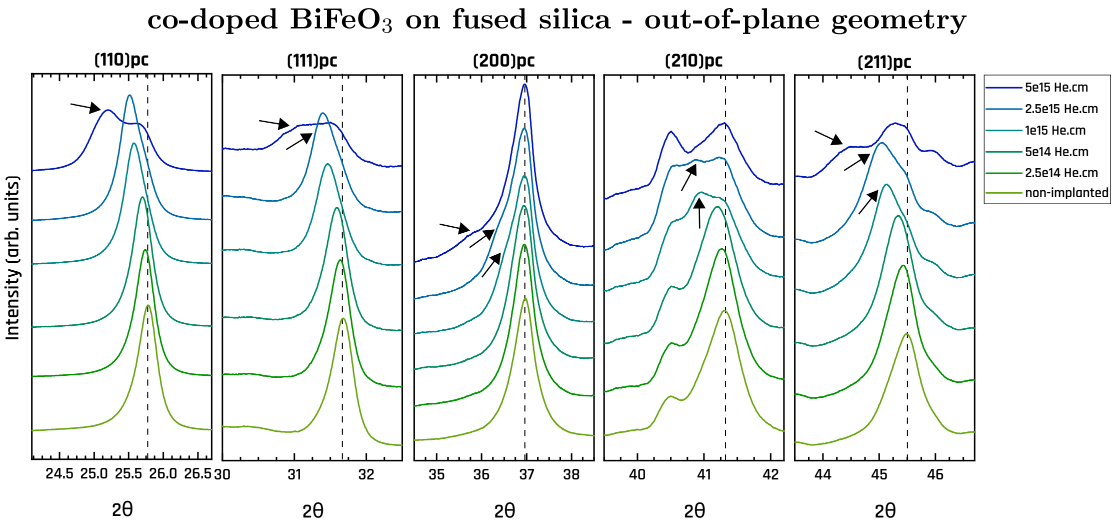


FIG. S8. Bragg Peaks measured on the co-doped $BiFeO_3$ film on fused silica, in the out-of-plane configuration. The arrows show the appearance of the new peaks.

## II. VISUALIZATION OF THE ZONES FROM A LINESCAN

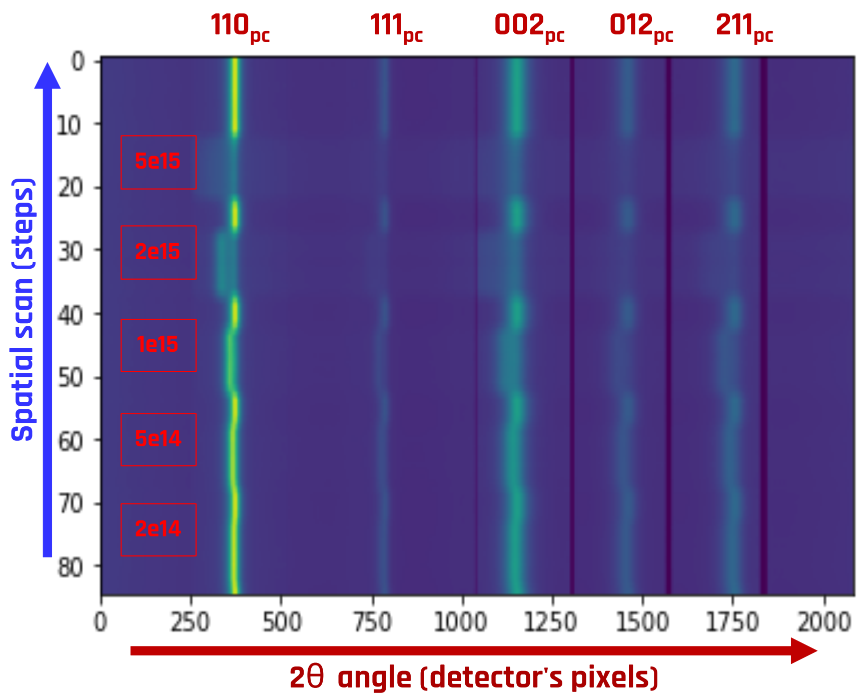


FIG. S9. XRD map showing the stacked spatial scans. It shows the evolution of the different Bragg peaks measures on $BiFeO_3$ /MgO co-doped film through the different implanted regions (and hence the different doses).

## III. EXAMPLE FOR A FIT OF A DIFFRACTION PATTERN

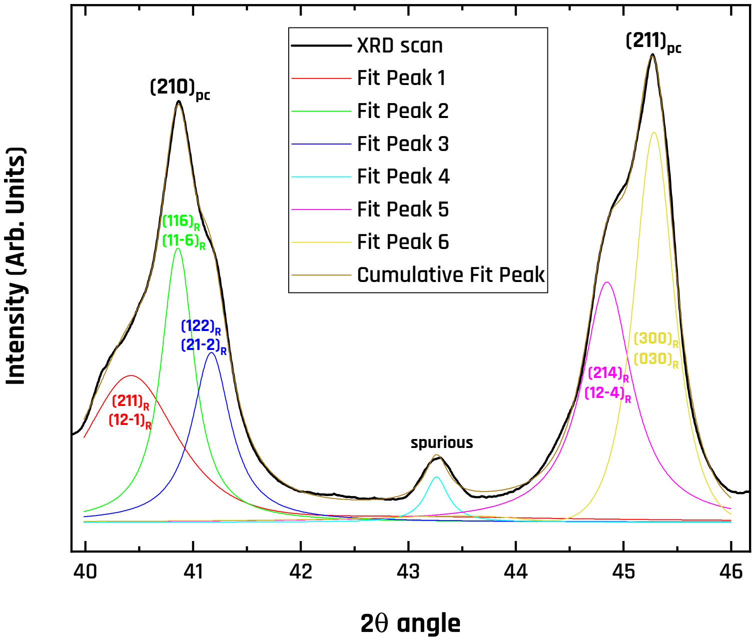


FIG. S10. Example of fits of the XRD scans with Voigt functions. Here the scan is a $\theta$–$2\theta$ scan done on the zone 3 (dose 1E15 He.cm$^{-2}$) of the BFO/MgO sample.

## IV. XRD PEAK WIDTHS AS A FUNCTION OF HE DOSE: REPRESENTATIVE EXAMPLES

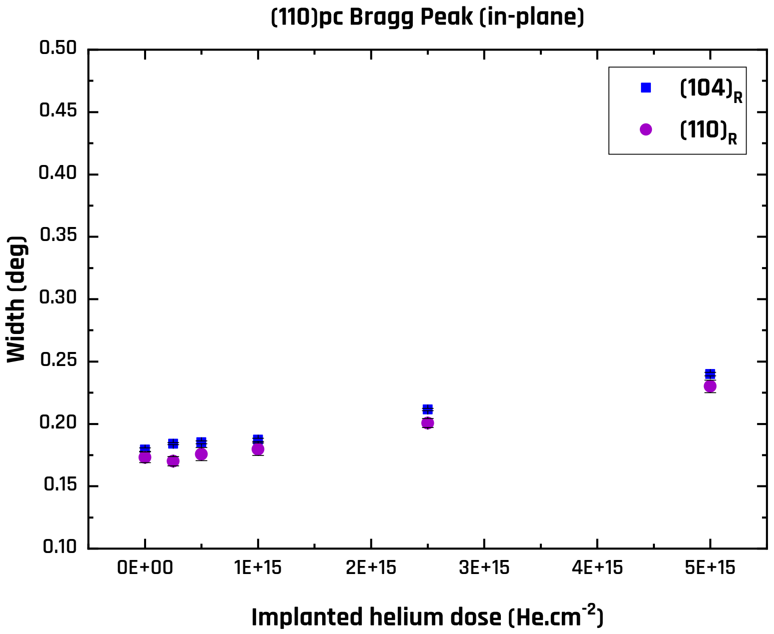


FIG. S11. Example of peak width behaviour under implantation, taken from the Voigt fit of the (110) Bragg peak in the IP configuration in BFO/MgO sample.

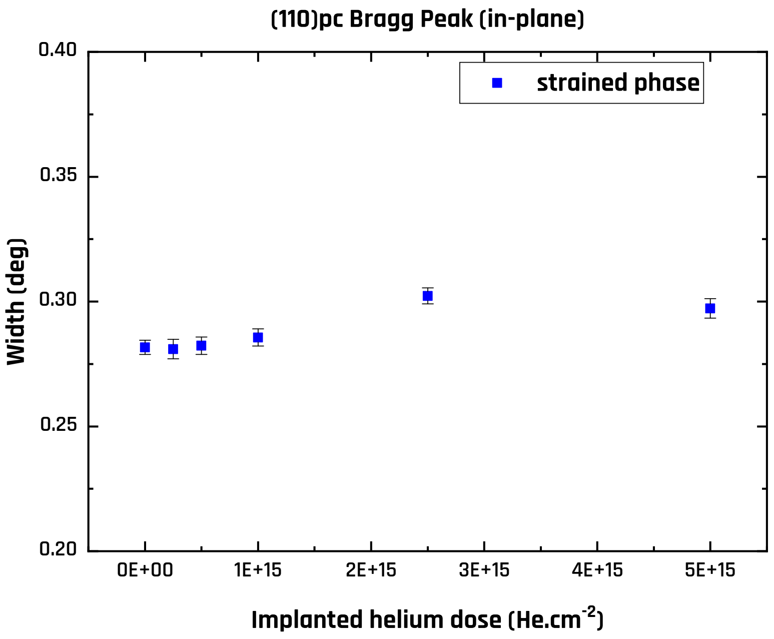


FIG. S12. Example of peak width behaviour under implantation, taken from the Voigt fit of the (110) Bragg peak in the IP configuration in BFMTO/MgO.

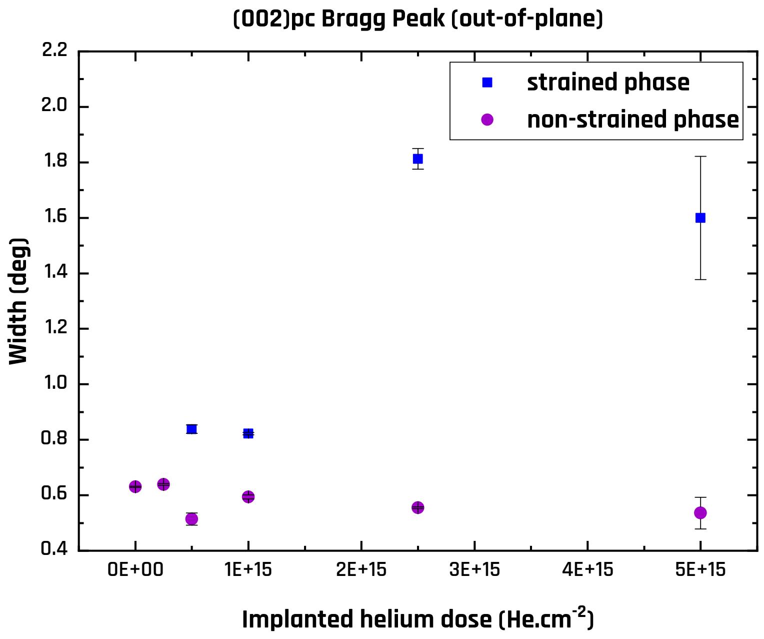


FIG. S13. Example of peak width behaviour under implantation, taken from the Voigt fit of the (002) Bragg peak in the OOP configuration in BFMTO/MgO.

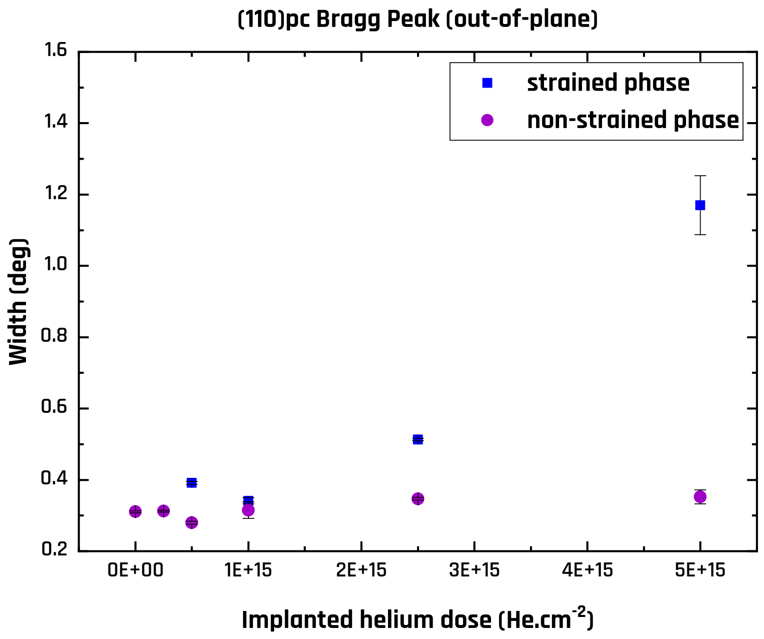


FIG. S14. Example of peak width behaviour under implantation, taken from the Voigt fit of the (110) Bragg peak in the OOP configuration in BFMTO/MgO.

## V. IRRELEVANCE OF A SMALL TILT FOR THE STRAIN VALUES

The substrate is a good quality single crystal with very intense but very thin Bragg peaks as measured for example by rocking curves in XRD (width of the order of 0.1° or less typically). Our thin films on the other hand are polycrystalline and show diffraction rings that are visible at all angles. A small tilt of 3° is enough to move away from the substrate peak while still capturing the signal of the film. The relative intensities of the peak may change if the film shows dome degree of preferred orientation, but this does not affect the peak positions needed for strain calculations.

By tilting the substrate, we are measuring an interplanar spacing $d$ along a direction that is slightly off with respect to the normal to the substrate surface. For an unstrained polycrystalline sample, this tilt is irrelevant because the XRD intensity is distributed on a sphere. For a strained film, it makes a difference in principle but in practice the error made on the lattice constants (and the strain) is very small. This can be visualized and estimated as detailed below.

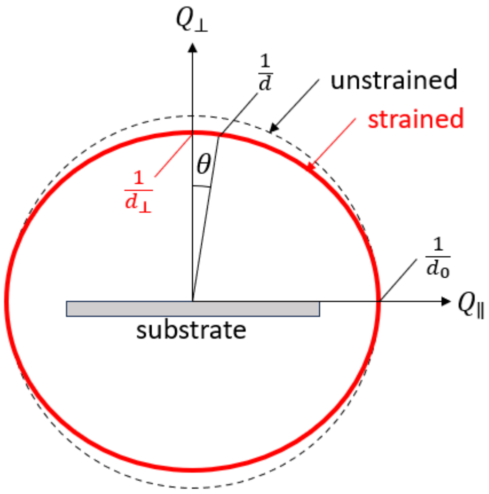


This sketch represents the distribution of XRD intensity in $Q$-space for a polycrystalline unstrained film (dashed circle with radius $1/d_0$) and for a film that is elongated along the direction normal to the substrate but clamped in the plane (solid red ellipse). With a "true" strain calculated as $\varepsilon = d_\perp/d_0 - 1$, and in the limit of a small $\theta$ angle, one can show that $d$ is given by $d = d_\perp(1 - \varepsilon\theta^2)$ and the "apparent" strain calculated with this value is $\varepsilon_{\text{app}} = \varepsilon(1 - \theta^2)$. With $\varepsilon$ of the order of a few % and $\theta = 3° = 0.052\,\text{rad}$, this difference is negligible. The small tilt therefore does not affect the strain values given in the paper.
